# Supplementary material for: Coevolution Maintains Diversity in the Stochastic "Kill the Winner" Model
Source: arXiv:1706.02666 source file (2017-06-08)
Supplement: Supplementary file 1 [file v1.6_supplemental_material.pdf]

# Coevolution Maintains Diversity in the Stochastic "Kill the Winner" Model Supplemental Material

This Supplemental Material describes simulations of an open coevolving ecosystem, as described briefly in the main text. We construct a species space to manifest the trade-off in the birth rate due to mutation. For the particular set of parameters used in the simulations, there are $M = 20$ distinct pairs of preys and predators that can potentially exist in the system. The birth rates are $\boldsymbol{b} = (0.05, 0.15, 0.25, 0.35, 0.45, 0.55, 0.65, 0.75, 0.85, 0.95, 1, 0.9, 0.8, 0.7, 0.6, 0.5, 0.4, 0.3, 0.2, 0.1)$. The 11th species has the highest birth rate and is the origin of trait expansion. Mutations of the first and last species generating mutants with negative birth rates are excluded from the model. Other parameters are $p_i \equiv p = 2$, $\beta_i \equiv \beta = 10$, $d_i \equiv d = 0.5$, and $e_{ij} \equiv e = 1$. The individual level reactions have the same form as Eq. (1) and (4) in the main text, with index $i = 1, 2, \ldots, M$. In the mean-field situation, the carrying capacity allows the coexistence of 13 pairs, with indices from 5 to 17, while the rest 7 species are forbidden. In the presence of demographic stochasticity, mutants can emerge in the forbidden region in the species space, although they can not develop a significant population size, limited by the high competition with other individuals. The number of coexisting pairs can be greater that the value 13 predicted by the mean-field calculation, and varies with time. As shown in the prey population time series in Fig. S1(a) and (b), a small mutation rate results in the alternation of dominating winners, and a large mutation rate generates coexistence with much smaller fluctuations. Figure S1 (c) and (d) show the distribution of prey population across all species as a function of the distance to the winner, defined as the most abundant strain. The red bar graph stands for a snapshot at a certain moment, and the blue one represents the average of the distribution over a long time interval. It's clear that a winner stands out at low mutation rate, while no one is significantly dominant at high mutation rate. Figure S1(e) shows the dependence of prey diversity, defined as the Shannon entropy, on the mutation rate. The three regions as seen in the CKtW model with fixed number of pairs in the main text are recovered.

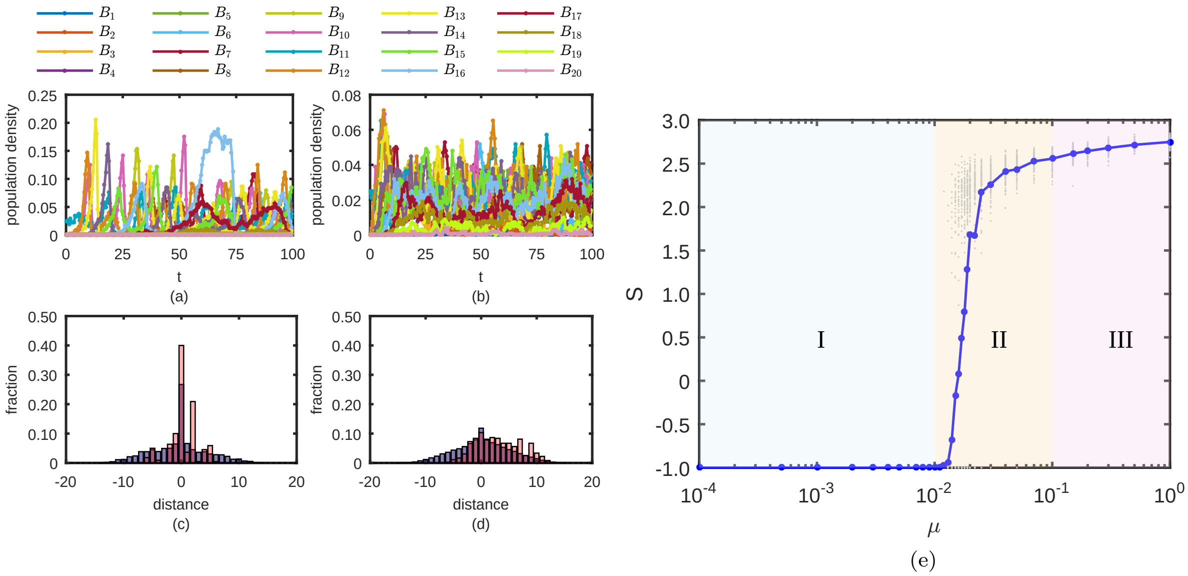


FIG. S1. Simulation results of the CKtW model with the number of coexisting species limited by the carrying capacity. Parameters used are $\boldsymbol{b} = (0.05, 0.15, 0.25, 0.35, 0.45, 0.55, 0.65, 0.75, 0.85, 0.95, 1, 0.9, 0.8, 0.7, 0.6, 0.5, 0.4, 0.3, 0.2, 0.1)$, $p_i \equiv p = 2$, $\beta_i \equiv \beta = 10$, $d_i \equiv d = 0.5$, and $e_{ij} \equiv e = 1$. The system size is $C = 1000$. Population is initiated in the fittest species and expands in the species space. (a) and (b) are prey population time series for small mutation rate $\mu_1 = \mu_2 \equiv \mu = 0.02$ and large mutation rate $\mu_1 = \mu_2 \equiv \mu = 0.5$, respectively. At small mutation rate, winners alternate with time and the population is localized to the winner species. At large mutation rate, all species coexist and the population distribution is roughly uniform in the mean-field allowed region, with some mutants leaked into the forbidden species. (c) and (d) show the prey population distribution across the species as a function of index distance from the winner strain, constructed from (a) and (b), respectively. The red bar graph is calculated at $t = 499.5$, after the transient regime. The blue one is the distribution averaged over 501 snapshots uniformly sampled between $t = 249.5$ and $t = 499.5$. For reference, the mean-field steady state predicts that species with indices from 5 to 17 coexist with equal abundance and that other species have zero population. The center bar at 0 distance is the population fraction of the most abundant strain. It's clear that a winner dominates at low mutation rate but not at the high one. (e) The dependence of prey Shannon entropy on the mutation rate, defined in the same way as in the main text. At low mutation, the system collapses due to extinction; at intermediate mutation, diversity increases rapidly with the rate; at high mutation, diversity stays near the maximum given by the deterministic steady state.
